# Supplementary material for: Cormorant: Covariant Molecular Neural Networks
Source: arXiv:1906.04015 source file (2019-11-25)
Supplement: Supplementary file 1 [file supplement_cglayers.tex]

\section{Covariant $\SO(3)$-vector layers}
\label{sec:cg_layers}

We discuss the specific implementation of the covariant CG layers acting on the $\SO(3)$-vector 
activations $F_i$. Our network is inspired by the $n \leq 3$-atom interactions described in the main text. 
In practice, computational limitations forced us to take only a subset of these operations, in particular:  
%The set of operations we include in our CG-layer is:
\begin{equation}
%\mathrm{CGLayer}(\{F_{i},\mathbf{r}_{ij}\})=
\bigg[
\underbrace{\Big(F_{i}\oplus\brBig{\sum_{j}\Upsilon_{ij}^{\left(1\right)}\otimescg F_{j}}\Big)}_{\textrm{one-body}}
\oplus\underbrace{\left(F_{i}\otimescg F_{i}\right)}_{\textrm{two-body}}
%\oplus\underbrace{\left(F_{i}\right)^{\otimescg 2}}_{\textrm{two-body}}
%\oplus\underbrace{\left(\sum_{j}F_{i}\otimescg\Upsilon_{ij}^{\left(3\right)}\otimescg F_{j}\otimescg F_{j}\right)}_{\textrm{three-body}}
\oplus\underbrace{\Big(\sum_{j}F_{i}\otimescg\Upsilon_{ij}^{\left(3\right)}\otimescg \left(F_{j}\right)^{\otimescg 2}\Big)}_{\textrm{three-body}}
\bigg] \cdot W
\end{equation}
%
%\begin{align*}
%\mathrm{CGLayer}(\{F_{i},\mathbf{r}_{ij}\})&=F_{i}\oplus(\sum_{j}\Upsilon_{ij}\otimescg F_{j})\oplus\left(F_{i}\otimescg F_{i}\right)\oplus\big((\sum_{j}F_{i}\otimescg\Upsilon_{ij}\otimescg F_{j})\otimescg F_{j}\big)\\&=\sum_{j}\left(\delta_{ij}\oplus\Upsilon_{ij}\oplus\delta_{ij}F_{i}\oplus\big(F_{i}\otimescg\Upsilon_{ij}\otimescg F_{j}\big)\right)\otimescg F_{j}
%\end{align*}
For computational tractability, we replace 
$F_{i}\otimescg\Upsilon_{ij}^{\left(3\right)}\otimescg F_{j}$ by $(F_{i}\cdot F_{j}) \otimescg\Upsilon_{ij}^{\left(3\right)}$ in the three-body term. This can be be done 
using the properties of the CG transformation to give a unitary redefinition of $W \rightarrow W^\prime$, 
followed by a projection into the subspace for which $\ell_{\rm max} = 0$. 
After some algebra, we arrive at the form of our $\mathrm{CGLayer}$:
\begin{equation}
\mathrm{CGLayer}(\{F_{i},\mathbf{r}_{ij}\}) = 
\Big[F_i \oplus 
\big( F_{i}\otimescg F_{i}\big) \oplus 
\Big(\sum_{j}\Big(\Upsilon_{ij}^{\left(1\right)}\oplus 
\big(F_{i}\cdot F_{j}\big) \Upsilon_{ij}^{\left(3\right)}\Big)\otimescg F_{j} \big)\Big] 
\cdot W^\prime
\label{eq:cglayer-mpnn}
\end{equation}
%This is the basic structure of the $\mathrm{CGLayer}$-s we use in our networks. 

%\subsubsection{Edge networks}
%\label{sec:edge_networks}

Structurally, \rf{eq:cglayer-mpnn} looks similar to a message passing neural network 
\citep{Gilmer2017}), where messages are CG-products acting on $\SO(3)$-vector activations. 
%$\mathcal{E}^{s}_{ij} = $
In this framework, the term 
\sm{\Upsilon_{ij}^{\left(\mathrm{edge}\right)}  = \Upsilon_{ij}^{\left(1\right)}\oplus\left(F_{i}\cdot F_{j}\right)\Upsilon_{ij}^{\left(3\right)}} 
looks like an ``edge network'' with $\SO(3)$-vector messages. %~(\cite{Riley2017}). 
Inspired by this connection, we generalize our architecture to 
\begin{equation}
%\mathrm{CGLayer}(\{F_{i},\mathbf{r}_{ij}\}) = 
%\Big[\sum_{j}\left(\delta_{ij}\oplus\delta_{ij}F_{i}\oplus \mathcal{E}^{s}_{ij}\right)\otimescg F_{j}\Big] \cdot W^\prime 
\mathrm{CGLayer}(\{F_{i},\mathbf{r}_{ij}\}) = 
\Big[
F_i \oplus \big( F_{i}\otimescg F_{i}\big) \oplus 
\big( \sum_{j} \Upsilon_{ij}^{\left(\mathrm{edge}\right),s} \otimescg F_{j} \big)\Big] \cdot W^\prime.
\label{eq:cglayer-edge}
\end{equation}
Following this idea, we can allow the edge network to be ``self-consistently'' updated based upon the value at the previous level: 
\m{\Upsilon_{ij}^{\left(\mathrm{edge}\right),s} \equiv \big[ \Upsilon_{ij}^{\left(\mathrm{edge}\right),s-1} \oplus \Upsilon_{ij}^{\left(1\right),s}\oplus\big(F_{i}\cdot F_{j}\big)\Upsilon_{ij}^{\left(3\right),s} \big] \cdot W_{\mathrm{edge}}} is a ``self-consistent'' amplitude.
In practice, we assume $\Upsilon_{ij}^{\left(1,3\right),s} \propto Y^\ell(\hat{\mathbf{r}}_{ij})$. We can therefore calculate the edge network by defining $\Upsilon_{ij}^{\left(\mathrm{edge}\right),s}  = \bigoplus_{\ell=0}^{\ell_{\rm max}} \mathcal{E}^{s,\ell}_{ij} Y^\ell(\hat{\mathbf{r}}_{ij})$, and then updating 
\sm{\mathcal{E}^{s}_{ij} = \bigl( \mathcal{E}^{s-1}_{ij} \oplus \mathcal{F}^{(1),s}_{ij} \oplus \mathcal{D}^{s}_{ij} \bigr) \cdot W_{\rm edge}}, 
where $\mathcal{D}^{s}_{ij} = (F_{i}\cdot F_{j})$. 

%This replacement results in a $\mathrm{CGLayer}$ architecture defined by

%where 

%is an edge network that accounts for both one-body aggregation and a limited form of three-body interactions.

%\subsubsection{Masks and local environments}
%\label{sec:marks_local}

The functions $\Upsilon_{ij}$ define the position dependence of the interaction between atoms $i$ and $j$. In chemical environments, atoms that are separated by a significant distance will not talk to each other. For this reason we include a soft mask $\Upsilon_{ij} \rightarrow m_{ij} \times \Upsilon_{ij}$, where $m_{ij} = \sigma((r_{\rm cut} - r_{ij}) / w)$, and $r_{\rm cut}$, $w$ are respectively learnable cutoffs and widths described below.
