# Supplementary material for: Cormorant: Covariant Molecular Neural Networks
Source: arXiv:1906.04015 source file (2019-11-25)
Supplement: Supplementary file 2 [file supplement_interactions.tex]

\section{General $n$-atom Interaction terms}

We now write the general form of the $n$-atom interactions described in the main text. 

\begin{equation}

\end{equation}
